# Supplementary material for: From Reward-Free Representations to Preferences: Rethinking Offline Preference-Based Reinforcement Learning
Source: arXiv:2606.01123 source file (2026-05-31)
Supplement: Supplementary file 1 [file appendix-C.tex]

% To be put in Section 4
\section{Reward-Free Representations for Preference-based Learning}

\subsection{Connecting RFRL with SimCLR Contrastive Learning}
We propose to leverage the FB representations pre-trained via RFRL in preference-based learning.
Let $\bar{\mathbf{F}}$ and $\bar{\mathbf{B}}$ denote the pre-trained forward and backward representations under the vanilla FB method.
We assume linear realizability of the reward function under the backward representation, \ie for each state-action pair $(s,a)$,
\begin{equation}
    r_{\bm{\psi}}(s,a):=\bar{\mathbf{B}}(s,a)^\top\bm{\psi}, 
\end{equation}
where $\bm{\psi}\in \mathbb{R}^d$.
Given this assumption, we can derive the corresponding latent vector $\bm{z}$ for the FB framework for each reward function as
\begin{equation}
    \bm{z}_{\bm{\psi}}^*=\mathbb{E}_{(s,a)\sim\rho}\big[\bar{\mathbf{B}}(s,a)r_{\bm{\psi}}(s,a)\big]=\mathbb{E}_{(s,a)\sim\rho}\Big[\bar{\mathbf{B}}(s,a)\big(\bar{\mathbf{B}}(s,a)^\top\bm{\psi}\big)\Big]=\underbrace{\Big(\mathbb{E}_{(s,a)\sim\rho}\Big[\bar{\mathbf{B}}(s,a)\bar{\mathbf{B}}(s,a)^\top\Big] \Big)}_{=:\mathbf{H}_{\mathbf{B}}}\bm{\psi},
\end{equation}
where $\mathbf{H}_{\mathbf{B}}$ is a $d\times d$ and non-negative definite matrix.
The above suggests that if $\mathbf{H}_{\mathbf{B}}$ is invertible, then there exists a bijection between $\bm{z}_{\bm{\psi}}^*$ and $\bm{\psi}$ as
\begin{equation}
    \bm{\psi}=\mathbf{H}_{\mathbf{B}}^{-1}\bm{z}_{\bm{\psi}}^*,\label{eq:bijection}
\end{equation}
for any reward function $r_{\bm{\psi}}$.

Now we are ready to connect RFRL under FB decomposition and the preference modeling.
Recall from~\Cref{sec:background} that we consider a general class of preference models 
\begin{equation}
    P_{\bm{\psi}}(\sigma^+ \succ \sigma^-)=\mu\big(R_{\bm{\psi}}(\sigma^+)-R_{\bm{\psi}}(\sigma^-)\big),
\end{equation}
where $\mu:\mathbb{R}\rightarrow[0,1]$ is a monotonically increasing function and $R_{\bm{\psi}}(\sigma)$ denotes the total expected reward associated with a trajectory $\sigma$ under the reward function $r_{\bm{\psi}}$.

%\begin{restatable}{prop}{simclr}
%Under 
%\end{restatable}
Then, we can rewrite the preference loss as
\begin{align}
    \mathcal{L}_{\text{pref}}(\bm{\psi})&=-\mathbb{E}_{(\sigma^+,\sigma^-)\sim \mathcal{D}_{\text{pref}}}\Big[\log\mu\big(R_\psi(\sigma^+)-R_\psi(\sigma^-)\big) \Big]\\
    &=-\mathbb{E}_{(\sigma^+,\sigma^-)\sim \mathcal{D}_{\text{pref}}}\bigg[\log \mu\Big( \sum_{t=1}^{k} \bar{\mathbf{B}}(s^+_t,a^+_t)^\top\bm{\psi}-\sum_{t=1}^{k} \bar{\mathbf{B}}(s^-_t,a^-_t)^\top \bm{\psi}\Big)\bigg]\\
    &=-\mathbb{E}_{(\sigma^+,\sigma^-)\sim \mathcal{D}_{\text{pref}}}\bigg[ \log \mu\big((\bm{z}^+_\sigma-\bm{z}^-_\sigma)^\top\bm{\psi}\big)\bigg].
\end{align}
Moreover, by the property in~\Cref{eq:bijection}, we can employ a change of variable and rewrite the preference loss in terms of latent vector $\bm{z}$ as follows
\begin{align}
     \mathcal{L}_{\text{pref}}(\bm{z})&=-\mathbb{E}_{(\sigma^+,\sigma^-)\sim \mathcal{D}_{\text{pref}}}\bigg[ \log \mu\big(\bm{z}^\top \mathbf{H}_{\mathbf{B}}^{-1}(\bm{z}^+_\sigma-\bm{z}^-_\sigma)\big)\bigg].\label{eq:pref loss in z}
\end{align}
Notably, under the standard Bradley-Terry preference model,~\Cref{eq:pref loss in z} takes the form as
\begin{align}
    \mathcal{L}_{\text{pref}}(\bm{z})=-\mathbb{E}_{(\sigma^+,\sigma^-)\sim \mathcal{D}_{\text{pref}}}\bigg[\log\bigg(\frac{\exp(\bm{z}^\top \mathbf{H}_{\mathbf{B}}^{-1}\bm{z}^+_\sigma)}{\exp(\bm{z}^\top \mathbf{H}_{\mathbf{B}}^{-1}\bm{z}^+_\sigma)+\exp(\bm{z}^\top \mathbf{H}_{\mathbf{B}}^{-1}\bm{z}^-_\sigma)}\bigg)\bigg].
\end{align}
Moreover, in the standard FB pre-training, we usually enforce two additional conditions: (i) We apply orthonomality for the backward representation and have $\mathbf{H}_{\mathbf{B}}=\mathbf{I}_d$. (ii) The FB framework presumes that the latent vector $\bm{z}$ is on the unit ball.
By using these two properties, we conclude that the preference loss exactly matches the SimCLR contrastive loss as
\begin{equation}
        \mathcal{L}_{\text{pref}}(\bm{z})=-\mathbb{E}_{(\sigma^+,\sigma^-)\sim \mathcal{D}_{\text{pref}}}\bigg[\log\bigg(\frac{\exp(\bm{z}^\top \bm{z}^+_\sigma)}{\exp(\bm{z}^\top \bm{z}^+_\sigma)+\exp(\bm{z}^\top \bm{z}^-_\sigma)}\bigg)\bigg].\label{eq:simclr loss}
\end{equation}

\subsection{Implications}

Based on the above derivation, there are two interesting implications.

\textbf{Why can reward-free representations lead to easier training than vanilla preference or reward modeling?} As the preference loss in~\Cref{eq:simclr loss} depends only on a low-dimensional latent vector $\bm{z}$, the optimization process can be much simpler than optimizing preference or reward models, which are implemented as neural networks in practice.

\textbf{Why can fine-tuning be helpful?} The aforementioned derivation depends on the assumption of linear realizability, and this may not exactly hold under the pre-trained backward representations. Through fine-tuning of FB-PbRL, the fine-tuned backward representations can better enforce this assumption.
